# Supplementary material for: Retina : Low-Power Eye Tracking with Event Camera and Spiking Hardware
Source: arXiv:2312.00425 source file (2024-04-17)
Supplement: Supplementary file 1 [file X_suppl.tex]

\clearpage
\setcounter{page}{1}
\maketitlesupplementary
\label{sec:suppl-materials}
 % Use alphabetical counters for sections

\setcounter{section}{0} % Reset section counter
We provide illustrative graphs for the processes behind dynamic time window slicing ( \cref{python_code}) and the temporal weighted-sum filter \cref{fig:filter_steps}. In addition, we include background information regarding the \ac{if} neuron model (\cref{sec:neuron_models}) and the hardware (\cref{sec:hardware}). Furthermore, in \cref{sec:firing_rate} we study the firing rate of different time window methods. Finally, \cref{sec:benchmark_eye_detection} provides a benchmark for future work on eye detection on Ini-30 in terms of centroid error, power consumption and latency.

\section{Dynamic Time Window}
\label{sec:dynamic_window}
For better illustration, in \cref{python_code}, we illustrate the operating principles and code to slice events into windows of dynamic time lengths. 

% \begin{figure}[h]
%     \centering
%     \includegraphics[trim={1.5cm, 4cm, 12.5cm, 2.5cm}, clip, width=\linewidth]{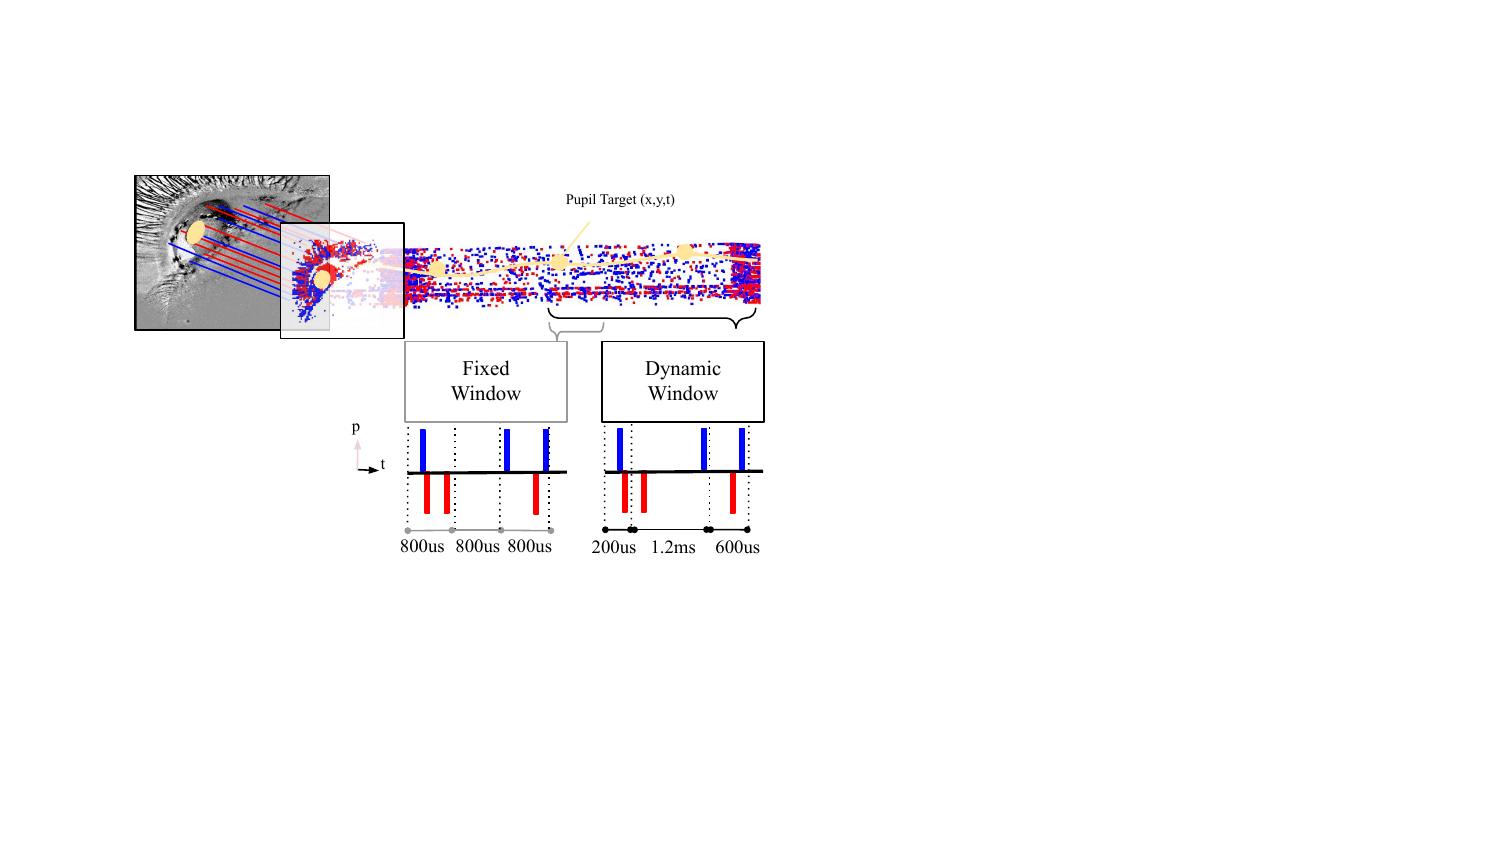} 
%     \caption{A graph illustrating the different techniques for slicing events (red, blue) in time: A) dt = $800us$, B) events count = $2$.}
%     \label{fig:dynamic-events-fixed-window}
% \end{figure}

\begin{lstlisting}[language=Python, caption=The code to dynamically slice event windows in time, label=python_code]
# data preparation
import numpy as np 
XYP=last_events_before_pupil_label
end_index = len(XYP) - 1
# event bins
tcwh=np.zeros(64,2,64,64))
for i in reversed(range(64)): 
 # events for time bin (i)
 x,y=last_unique_evs(XYP[:end_index,:2],N)
 start_index=end_index-len(x)
 p=XYP[start_index:end_index]
 # add events for i
 np.add.at(tcwh[i,0],(x[p==0],y[p==0]),1)
 np.add.at(tcwh[i,1],(x[p==1],y[p==1]),1) 
 # recover 1-bit event channel
 tcwh[i,0][tcwh[i,1]>=tcwh[i,0]]=0 
 tcwh[i,1][tcwh[i,1]<tcwh[i,0]]=0
 tcwh[i]=tcwh[i].clip(0, 1) 
 # move index
 end_index = start_index   
\end{lstlisting}

\section{Neuron Models}
\label{sec:neuron_models}
The \ac{if} neuron model, operating after every convolution layer, is characterized by a straightforward mathematical formulation. It involves the integration of incoming synaptic inputs (convolution operations) and the generation of a spike once a certain membrane potential threshold is reached. The dynamics of the \ac{if} neuron are described by the following differential equation:
\begin{equation}
\tau_m \frac{dV}{dt} = -V(t) + R_m I_{\text{syn}}(t)
\end{equation}

where $V(t)$ is the membrane potential at time $t$, $\tau_m$ is the membrane time constant, $R_m$ is the membrane resistance, and $I_{\text{syn}}(t)$ represents the synaptic input current. The neuron fires when $V(t)$ surpasses a predefined threshold $V(th)=1$, at which point the membrane potential is reset to a resting value $V(reset)=0$. One of the key features of the \ac{if} neuron model is its integration mechanism for incoming synaptic inputs. The synaptic input $Isyn(t)$ is often modeled as a sum of weighted contributions from different synapses:

\begin{equation}
I_{\text{syn}}(t) = \sum_{j} w_j \cdot I_j(t - t_j)
\end{equation}

where $w_j$ represents the synaptic weight, $I_j(t - t_j)$ is the synaptic input spike train arriving at time $t$ from synapse $j$ with a spike at $t_j$.

\begin{figure*}[h]
    \centering
    \includegraphics[trim={0cm, 2cm, 0cm, 1.1cm}, clip, width=\linewidth]{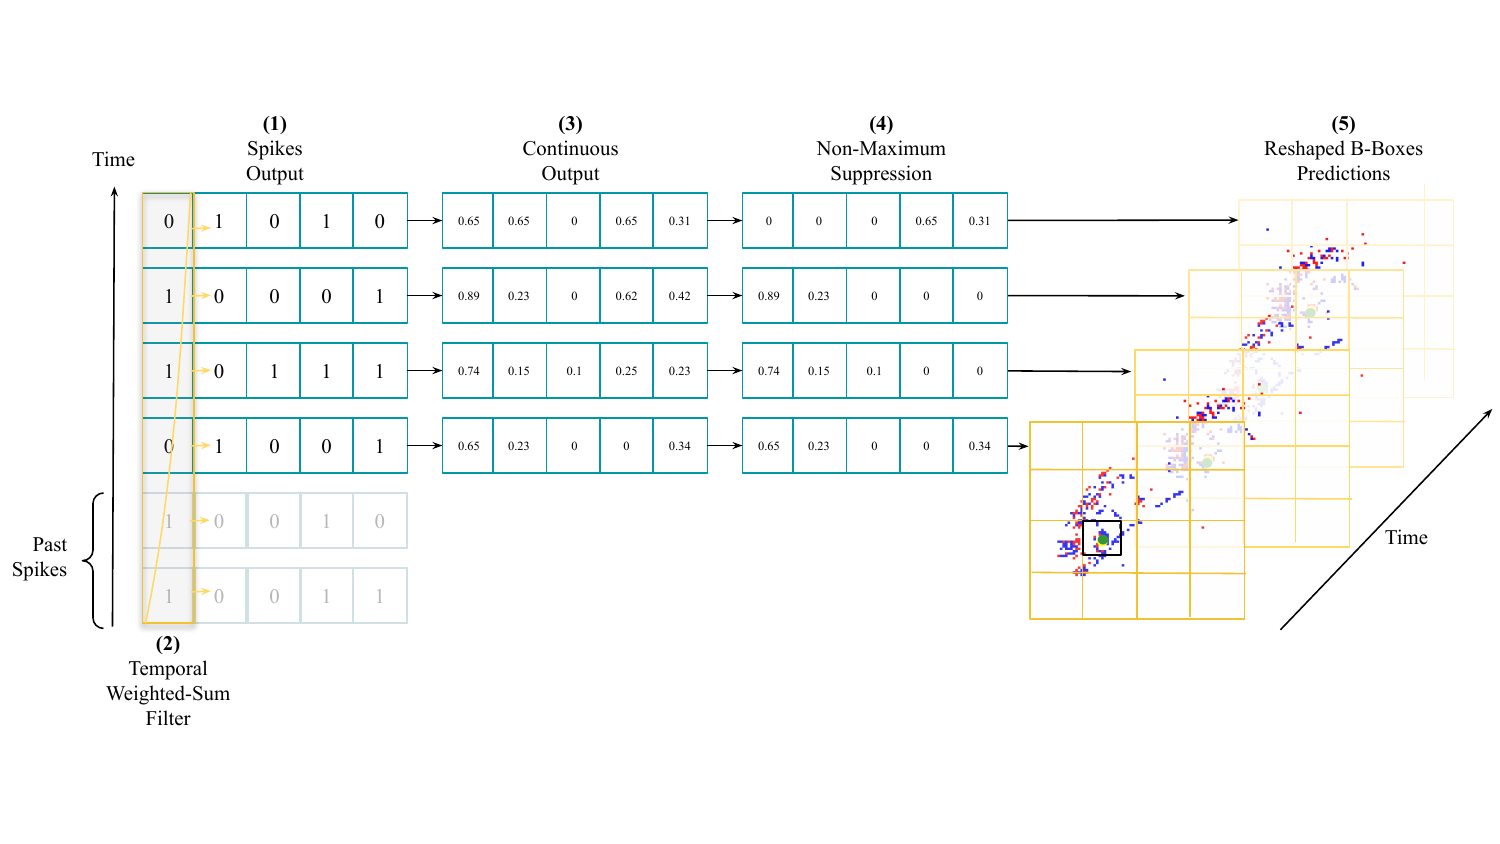}
    \caption{Overview of the steps involved in the conversion of spikes to bounding boxes. The output spikes 1) are multiplied to a temporal weighted sum filter 2). Next, only during training, the continuous output 3) is zeroed in cells where bounding boxes were non-existent in the target 4). Finally the centroid of the predicted bounding box is used to find the coordinate of the pupil 5).}
    \label{fig:filter_steps}
\end{figure*}

\section{Hardware Description}

\ac{speck} is equipped with nine cores with different kernel and neuron memory limitations, see \cref{tab:cores}.
\label{sec:hardware}
\begin{table}[htbp]  
    \centering
    \caption{The memory limits of each core in  \ac{speck} are reported in kibibyte (1 Ki = 1024 bytes).}
    \label{tab:cores}
    \small
    \begin{tabular}{c|c|c}
        \toprule
        Core ID & $K_{MT}$ (Ki) & $N_{M}$ (Ki) \\
        \midrule
        0 & 16  & 64  \\
        1 & 16  & 64  \\
        2 & 16  & 64  \\
        3 & 32  & 32  \\
        4 & 32  & 32  \\
        5 & 64  & 16  \\
        6 & 64  & 16  \\
        7 & 16 & 16  \\
        8 & 16 & 16  \\
        \bottomrule
    \end{tabular}  
\end{table}

 \section{Firing Rate}
\label{sec:firing_rate}
In \cref{tab:firing_rates}, we provide insights into the firing behavior of the \ac{snn} at different network depths. 
Results show the dynamic time window of events has considerably lower firing rate in the first layer. For the rest of the layers, there is no significant variation between the spiking activity across different slicing methods, different time window or different event counts. 

\begin{figure}[h]
    \centering
    \begin{tabular}{c}
        \begin{subfigure}{0.8\linewidth}
            \centering
            \includegraphics[trim={0cm, 0cm, 0cm, 0cm}, clip, width=\linewidth]{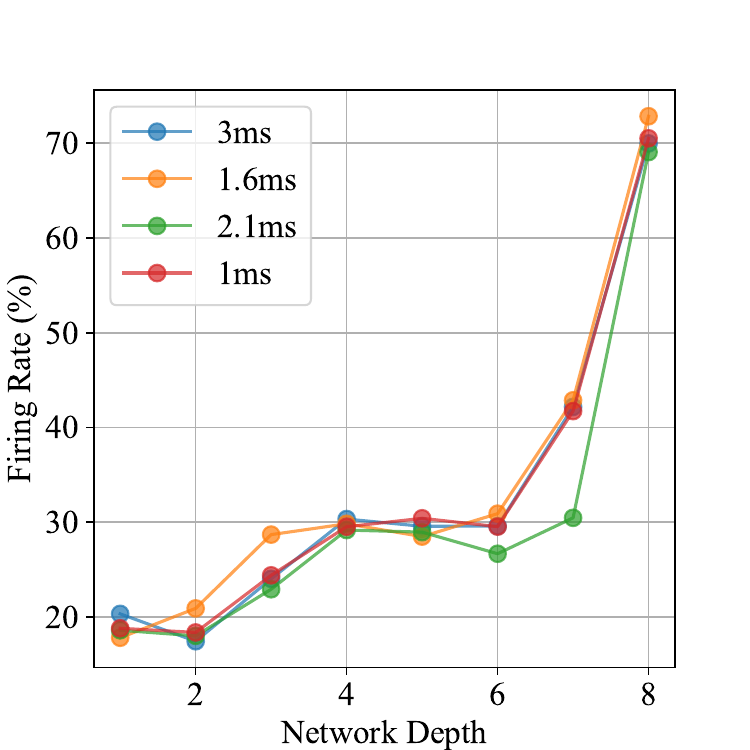}
            \caption{Firing Rates of the Fixed Time Window.}
        \end{subfigure} \\
        \begin{subfigure}{0.8\linewidth}
            \centering
            \includegraphics[trim={0cm, 0cm, 0cm, 0cm}, clip, width=\linewidth]{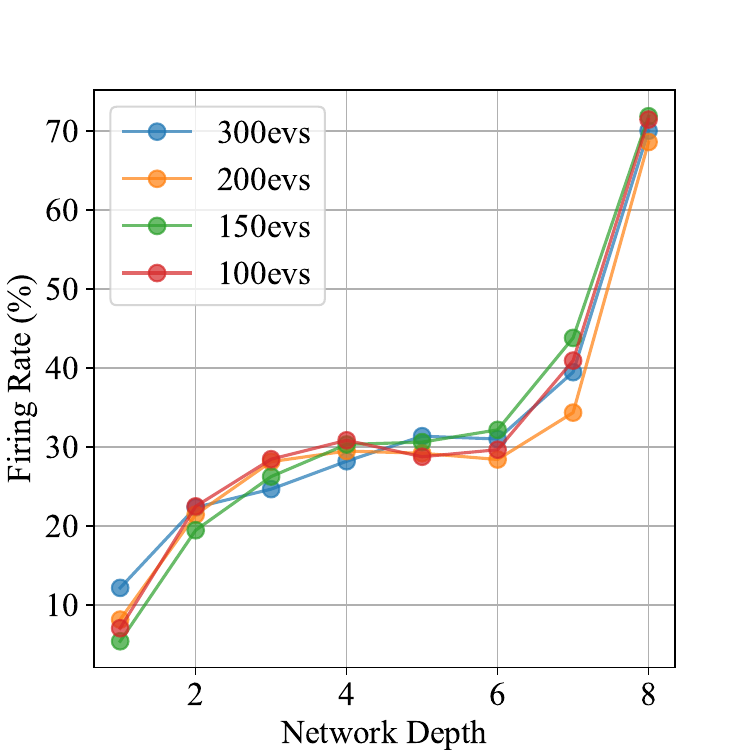}
            \caption{Firing Rates of the Dynamic Time Window.}
        \end{subfigure} \\
    \end{tabular}
    \caption{The firing rates of the trained \ac{snn} at different network depths with different slicing methods and time windows.}
    \label{tab:firing_rates}
\end{figure}

At the beginning, the network can save energy consumption by having less than 30\% spikes generated per layer. The higher firing rates at the ends might be the results of directly converting spikes to bounding boxes coordinates [0,1]. 

\section{Additional Results}
\label{sec:benchmark_eye_detection}

\subsection{Benchmark Eye Detection on Ini-30}

In this section material, we consider the simpler task of eye detection and provide two benchmarks for future work on Ini-30. 

\subsubsection{Eye Detection Architectures}

For pupil detection, we evaluate models which do not possess a temporal dimension. In this task, we evaluate a standard \ac{cnn} and compared it with an edge-version of the yolo network \cite{redmon2016look}, namely Tinyissimo-YoloV8 (TY-V8) \cite{moosmann2023ultraefficient}, which has been proven to be well-suited for deployment on ultra-low power microcontrollers. Since pupil detection has only one class we reduced the depth multiple in \cite{moosmann2023ultraefficient} to 0.1 (versus 0.3), the layer channel multiple of 0.1 (versus 0.18), reduced the number of predictions heads from 16 to 1 and thus obtained a model of around 30k parameters (vs 1M for Tinyissimo-YoloV8-B). In these experiments, we accumulated events with linear decay with time windows of $3ms$.

\subsubsection{Centroid Error}
In \cref{table:mac-params-detection}, we evaluate the efficiency of these models in terms of number of \ac{mac} and parameters and report the centroid error on the validation set after 520k steps. The \ac{cnn} was trained with the original resolution and showed an error of 5px. In relative terms (RError), this corresponds to 0.5px in the 64x64 array. TY-V8 was instead trained on a 128x128 resolution and resulted in a 3.5px error (1.75px in 64x64). Both of these models are relative more precise than Retina, however neither of these architectures can be deployed on neuromorphic hardware.

\begin{table}[h]
\centering
\caption{The benchmark for network complexity and error for pupil detection (64x64).}
\label{table:mac-params-detection}
\small
\begin{tabular}{c|c|c|c}
\toprule
Model &   MAC (M)  $\downarrow$  & Params (k)  $\downarrow$  & Error (px)  $\downarrow$  \\
\midrule 
\ac{cnn} (Baseline)  & 150 & 120  & 0.5 \\
TY-V8 & 0.42 & 28 & 1.75 \\ 
\bottomrule
\end{tabular}
\end{table}

% In \cref{tab:tiny-yolo-v8}, we provide qualitative insights into the TY-V8 network performance. Given that all the prediction are independent, the model may lose track of the pupil, however when compared to Retina this model performs equally well. 

% \begin{figure}[h]
%     \centering 
%         \includegraphics[trim={0cm, 0cm, 0cm, 0cm}, clip, width=\linewidth]{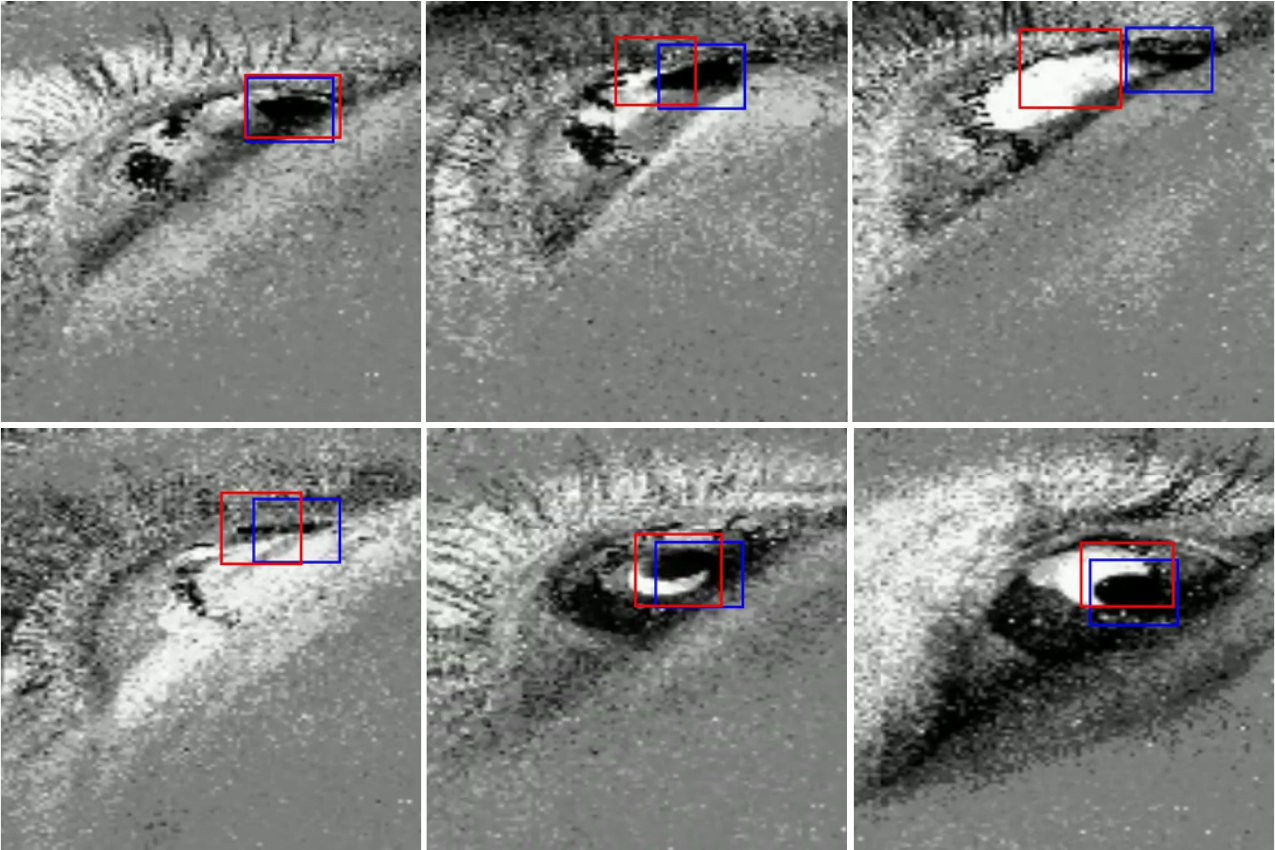}
%         \caption{Qualitative results with TY-V8 for Pupil Detection on Ini-30}
%     \label{tab:tiny-yolo-v8}
% \end{figure}

\subsubsection{Latency \& Power}
In \cref{table:power-latency}, we evaluate the power consumption of the eye detection models on two processors. We deployed the first large \ac{cnn} on an Intel® Core™ i7 Processor and the second TY-V8 on the GAP9 RISC-V Processor from GreenWaves.

\begin{table}[h]
\centering
\caption{The benchmark for latency (mS) and power (mW) for pupil detection.}
\label{table:power-detection}
\small
\begin{tabular}{c|c|c|c}
\toprule
Model &  Platform & Latency [ms]  $\downarrow$  & Power  $\downarrow$  \\
\midrule 
\ac{cnn} (Baseline)   & i7 CPU & 3.0  & 225 W \\
TY-V8 & GAP9 & 6.1 & 94 mW \\ 
\bottomrule
\end{tabular}
\end{table}

 Our results indicates higher power consumption (in particular in i7) and comparable latency w.r.t. \ac{speck}.

% 
% To split the supplementary pages from the main paper, you can use \href{https://support.apple.com/en-ca/guide/preview/prvw11793/mac#:~:text=Delete%20a%20page%20from%20a,or%20choose%20Edit%20%3E%20Delete).}{Preview (on macOS)}, \href{https://www.adobe.com/acrobat/how-to/delete-pages-from-pdf.html#:~:text=Choose%20%E2%80%9CTools%E2%80%9D%20%3E%20%E2%80%9COrganize,or%20pages%20from%20the%20file.}{Adobe Acrobat} (on all OSs), as well as \href{https://superuser.com/questions/517986/is-it-possible-to-delete-some-pages-of-a-pdf-document}{command line tools}.

% \begin{table}[h]
% \centering
% \caption{Performance with different \ac{dvs} resolutions.}
% \label{table:centroid-error}
% \small
% \begin{tabular}{c|c|c|c}
% \toprule
% \multirow{2}{*}{Method} &\multirow{2}{*}{Resolution} & \multicolumn{2}{c}{Error ($\pm$) on Test Dataset  $\downarrow$ } \\ \cline{3-4}
%  & & Synthetic \cite{chen20233et} & Ini-30 (Ours) \\ 
%  \midrule
% 3ET \cite{chen20233et} & \multirow{3}{*}{64x64x2}  & \multirow{3}{*}{N/A} &  4.48 ($\pm$ 1.94) \\
% Retina  w/o $L_{box}$ &  &  &  5.89 ($\pm$ 1.71) \\
% Retina  & &  &   \textbf{3.24 ($\pm$ 0.79)} \\  \midrule
 
% 3ET \cite{chen20233et} &  \multirow{3}{*}{128x128x1} & 9.37 ($\pm$ 4.86) &  9.04 ($\pm$ 4.69) \\
% Retina  w/o $L_{box}$ & & 11.15 ($\pm$ 3.02) & 12.73 ($\pm$ 4.18)\\
% Retina  & & \textbf{8.92 ($\pm$ 3.45)} &  \textbf{7.21 ($\pm$ 3.15)} \\
% \bottomrule
% \end{tabular}
% \end{table}
